# Supplementary material for: BAR: A Backward Reasoning based Agent for Complex Minecraft Tasks
Source: arXiv:2505.14079 source file (2025-05-30)
Supplement: Supplementary file 1 [file observation_space.tex]

\begin{table*}[!htb]
\caption{Details of the action space in Minecraft and the encapsulation of used steps in our experiments.}
\begin{tabular}{ccp{7cm}}
\hline
\textbf{Observation} & \textbf{Shape} & \textbf{Description}                                                                                          \\ \hline
point\_of\_view            & (360,640,3)    & The RGB imag observed by agent                                                                                \\ \hline
player\_position           & (3,)           & The 3D coordinates of the agent's location                                                                    \\ \hline
inventory                  & (36,)          & The items and corresponding quantities in the agent's inventory. There are totally 36 slots in the inventory. \\ \hline
execute\_flag              & (1,)           & The return information for each step, 1 represents success, 0 represents   failure.                           \\ \hline
\end{tabular}

\label{tab:observation_space}
\end{table*}
