# Supplementary material for: BAR: A Backward Reasoning based Agent for Complex Minecraft Tasks
Source: arXiv:2505.14079 source file (2025-05-30)
Supplement: Supplementary file 2 [file ores_distribution_paras.tex]

\begin{table*}[!htb]
\caption{Parameters for the sparse distribution algorithm of rare ores}
\begin{tabular}{lccc}
\hline
\multicolumn{1}{c}{\textbf{Parameter}}                & \textbf{Gold Ores} & \textbf{Redstone Ores} & \textbf{Diamond Ores} \\ \hline
Circle Nums                                      & 4                  & 4                      & 4                     \\
Circle Thickness                                 & 3                  & 3                      & 3                     \\
Distance between Circles                         & 6                  & 6                      & 6                     \\
Distance between First Circle and Starting Point & 10                 & 10                     & 10                    \\
Filling Ratio                                    & 0.2                & 0.2                    & 0.125                 \\
Unit Length                                      & 2                  & 2                      & 2                     \\ \hline
\end{tabular}

\label{tab:ores_distribution_paras}
\end{table*}
